# Supplementary material for: Concise Read-Only Specifications for Better Synthesis of Programs with Pointers -- Extended Version
Source: arXiv:2001.10723 source file (2020-01-29)
Supplement: Supplementary file 2 [file appendix-old.tex]

% Pre-Strengthening and Post-Weakening with imm - enables the verification of
% read only methods from a context which has write permission:
% \ac{BELOW DOESN'T HOLD ANYMORE }


% \begin{mathpar}
%   \inferrule[]
%   {\mcode{
%       P\iann{\mut} \Rightarrow P'\iann{\bimm{\mut}}
%       \quad
%       \{P'\iann{\bimm{\mut}}\} ~c~ \{Q'\iann{\bimm{\mut}}\}
%       \quad
%       Q'\iann{\bimm{\mut}} \Rightarrow Q\iann{\mut}
%     }}
%   {\mcode{
%       \{P\iann{\mut}\} ~c~ \{Q\iann{\mut}\}
%     }}
%     \end{mathpar}

\input{optimizations}


\noindent{\emph{\bf Synthesis for \ref{eq:pick}.}}.
First attempt:\\
{\centering
  \tiny{
\begin{prooftree}
%%
%%
  \Hypo[]
  {
    \begin{array}{c}
      \mcode{\neg{(\subann{\bimm{\ann}}{\mut})}}
    \end{array}
  }
%%
%%
\Infer1[\writer]
{
  \begin{array}{c}
    \mcode{\set{x, y};
      \trans
      {\asn{ \ispointsto{y}{30}{\bimm{\ann}}}}
      {\asn{ \ispointsto{y}{239}{\bimm{\ann}} }}
      {\prog_3}}
    \\[3pt]
    \mcode{\prog_2 = \prog_3}
  \end{array}
}
%%
%%
\Infer1[\framer]
{
  \begin{array}{c}
    \mcode{\set{x, y};
      \trans
      {\asn{ \gbm{\ispointsto{x}{239}{\mut}} \sep \ispointsto{y}{30}{\bimm{\ann}}}}
      {\asn{ \gbm{\ispointsto{x}{239}{\mut}} \sep \ispointsto{y}{239}{\bimm{\ann}} }}
      {\prog_2}}
  \\[3pt]
  \mcode{[\subs{z}{239}]\ispointsto{x}{z}{\mut} = \ispointsto{x}{239}{\mut}}
  \qquad
  \mcode{\prog_1 = \prog_2}
\end{array}
}
%%
%%
\Infer1[\hunir]
{
  \mcode{
    \set{x, y};
    \trans
    {\asn{ \gbm{\ispointsto{x}{239}{\mut}} \sep \ispointsto{y}{30}{\bimm{\ann}}}}
    {\asn{ \gbm{\ispointsto{x}{z}{\mut}} \sep \ispointsto{y}{z}{\bimm{\ann}} }}
    {\prog_1}
}
}
\end{prooftree}
}}

Second attempt (search strategy: if there are multiple options of
unification, favor the unification of the immutable heap first):\\
{\centering
  \tiny{
\begin{prooftree}
%%
%%
  \Infer0[\empr \text{with } {$\prog_5$ = \tt{skip}} ]
  {
    \begin{array}{c}
      \mcode{\set{x, y};
        \trans
        {\asn{ \emp }}
        {\asn{ \emp }}
        {}}
      \\[3pt]
      \mcode{\prog_4 =  \prog_5}
    \end{array}
  }
  %%
  %%
  \Infer1[\framer]
  {
    \begin{array}{c}
      \mcode{\set{x, y};
        \trans
        {\asn{ \gbm{\ispointsto{x}{30}{\mut}}}}
        {\asn{ \gbm{\ispointsto{x}{30}{\mut} }}}
        {\prog_4}}
      \\[3pt]
      \mcode{\prog_3 = \Letz {\deref{x}} = 30; \prog_4}
    \end{array}
  }
%%
%%
\Infer1[\writer]
{
  \begin{array}{c}
    \mcode{\set{x, y};
      \trans
      {\asn{ \gbm{\ispointsto{x}{239}{\mut}}}}
      {\asn{ \gbm{\ispointsto{x}{30}{\mut} }}}
      {\prog_3}}
    \\[3pt]
    \mcode{\prog_2 = \prog_3}
  \end{array}
}
%%
%%
\Infer1[\framer]
{
  \begin{array}{c}
    \mcode{\set{x, y};
      \trans
      {\asn{ {\ispointsto{x}{239}{\mut}} \sep \gbm{\ispointsto{y}{30}{\bimm{\ann}}}}}
      {\asn{ {\ispointsto{x}{30}{\mut}} \sep \gbm{\ispointsto{y}{30}{\bimm{\ann}}}}}
      {\prog_2}}
  \\[3pt]
  \mcode{[\subs{z}{30}]\ispointsto{y}{z}{\bimm{\ann}} = \ispointsto{y}{30}{\bimm{\ann}}}
  \qquad
  \mcode{\prog_1 = \prog_2}
\end{array}
}
%%
%%
\Infer1[\hunir]
{
  \mcode{
    \set{x, y};
    \trans
    {\asn{ {\ispointsto{x}{239}{\mut}} \sep \gbm{\ispointsto{y}{30}{\bimm{\ann}}}}}
    {\asn{ {\ispointsto{x}{z}{\mut}} \sep \gbm{\ispointsto{y}{z}{\bimm{\ann}} }}}
    {\prog_1}
}
}
\end{prooftree}
}}

\ac{For the above program, is there any way to tweak the rules to synthesize
\mcode{\Letz {\tt{v}} = {\deref{y}}; \Letz {\deref{x}} = v; } instead?}


% \input{fig/simple-eq}
